# Supplementary material for: Zero-shot Triplet Extraction by Template Infilling
Source: arXiv:2212.10708 source file (2023-09-20)
Supplement: Supplementary file 1 [file supplementary_materials.tex]

\section{List of All Templates}
\begin{center}
\begin{small}
\begin{longtable}[ht]{p{1in}|p{0.4in}|p{1.8in}|p{2.5in}}
\hline
\multicolumn{1}{c}{\textbf{Relation}} & \multicolumn{1}{c}{\textbf{Id}} & \multicolumn{1}{c}{\textbf{Template}} & \multicolumn{1}{c}{\textbf{Description}} \\ \hline
applies to jurisdiction & P1001 & \texttt{[H]} is a legal term in \texttt{[T]} . & the item (institution, law, public office, public register...) or statement belongs to or has power over or applies to the value (a territorial jurisdiction: a country, state, municipality, ...) \\
field of work & P101 & \texttt{[H]} works in the field of \texttt{[T]} . & specialization of a person or organization \\
member of political party & P102 & \texttt{[H]} is a member of political party \texttt{[T]} . & the political party of which a person is or has been a member or otherwise affiliated \\
taxon rank & P105 & \texttt{[H]} is a taxon rank of \texttt{[T]} . & level in a taxonomic hierarchy \\
occupation & P106 & \texttt{[H]}'s job is \texttt{[T]} . & occupation of a person \\
league & P118 & \texttt{[T]} is a league of \texttt{[H]} . & league in which team or player plays or has played in \\
publisher & P123 & \texttt{[H]} is published by \texttt{[T]} . & organization or person responsible for publishing books, periodicals, printed music, podcasts, games or software \\
owned by & P127 & \texttt{[H]} is owned by \texttt{[T]} . & owner of the subject \\
instrument & P1303 & \texttt{[H]} plays \texttt{[T]} . & musical instrument that a person plays or teaches or used in a music occupation \\
located in the administrative territorial entity & P131 & \texttt{[H]} is located in the administrative territorial entity of \texttt{[T]} . & the item is located on the territory of the following administrative entity. \\
participant in & P1344 & \texttt{[H]} is a participant in \texttt{[T]} . & event in which a person or organization was/is a participant \\
winner & P1346 & \texttt{[T]} is a winner of \texttt{[H]} . & winner of a competition or similar event, not to be used for awards \\
movement & P135 & \texttt{[H]} is part of movement \texttt{[T]} . & literary, artistic, scientific or philosophical movement or scene associated with this person or work \\
genre & P136 & \texttt{[T]} is a genre of \texttt{[H]} . & creative work's genre or an artist's field of work \\
operator & P137 & \texttt{[T]} is an operator of \texttt{[H]} . & person, profession, or organization that operates the equipment, facility, or service \\
religion & P140 & \texttt{[H]}'s religion is \texttt{[T]}. & religion of a person, organization or religious building, or associated with this subject \\
licensed to broadcast to & P1408 & \texttt{[H]} is lisensed to broadcast to \texttt{[T]} . & place that a radio/TV station is licensed/required to broadcast to \\
nominated for & P1411 & \texttt{[H]} is nominated for \texttt{[T]} . & award nomination received by a person, organisation or creative work \\
heritage designation & P1435 & \texttt{[H]} is designated as heritage by \texttt{[T]} . & heritage designation of a cultural or natural site \\
contains administrative territorial entity & P150 & \texttt{[H]} contains administrative territorial entity \texttt{[T]} . & direct subdivisions of an administrative territorial entity \\
follows & P155 & \texttt{[H]} follows \texttt{[T]} . & immediately prior item in a series of which the subject is a part \\
followed by & P156 & \texttt{[H]} is followed by \texttt{[T]} . & immediately following item in a series of which the subject is a part \\
headquarters location & P159 & \texttt{[H]} is headquartered in \texttt{[T]} . & city, where an organization's headquarters is or has been situated \\
performer & P175 & \texttt{[T]} is a performer of \texttt{[H]} . & actor, musician, band or other performer associated with this role or musical work \\
manufacturer & P176 & \texttt{[H]} is manufactured by \texttt{[T]} . & manufacturer or producer of this product \\
crosses & P177 & \texttt{[H]} crosses \texttt{[T]} . & obstacle (body of water, road, railway...) which this bridge crosses over or this tunnel goes under \\
developer & P178 & \texttt{[H]} is developed by \texttt{[T]} . & organization or person that developed the item \\
after a work by & P1877 & \texttt{[H]} after a work by \texttt{[T]} . & artist whose work strongly inspired/ was copied in this item \\
participating team & P1923 & \texttt{[T]} is a participating team in \texttt{[H]} . & like Participant but for teams \\
located in or next to body of water & P206 & \texttt{[H]} is located in or next to body of water \texttt{[T]} . & body of water on or next to which a place is located \\
competition class & P2094 & \texttt{[H]} is in the competition class \texttt{[T]} . & official classification by a regulating body under which the subject (events, teams, participants, or equipment) qualifies for inclusion \\
father & P22 & \texttt{[T]} is a father of \texttt{[H]} . & male parent of the subject \\
military branch & P241 & \texttt{[H]} is a military branch of \texttt{[T]} . & branch to which this military unit, award, office, or person belongs \\
mother & P25 & \texttt{[T]} is a mother of \texttt{[H]} . & female parent of the subject \\
spouse & P26 & \texttt{[H]} is a spouse of \texttt{[T]} . & the subject has the object as their spouse \\
record label & P264 & \texttt{[H]} is represented by the record label \texttt{[T]} . & brand and trademark associated with the marketing of subject music recordings and music videos \\
country of citizenship & P27 & \texttt{[H]} is citizen of \texttt{[T]} . & the object is a country that recognizes the subject as its citizen \\
location & P276 & \texttt{[H]} is located in \texttt{[T]} . & location of the object, structure or event. \\
operating system & P306 & \texttt{[H]}'s operating system is \texttt{[T]} . & operating system (OS) on which a software works or the OS installed on hardware \\
sibling & P3373 & \texttt{[H]} is a sibling of \texttt{[T]} . & the subject and the object have the same parents (brother, sister, etc.) \\
sports season of league or competition & P3450 & \texttt{[H]} is a sports season of league or competition of \texttt{[T]} . & property that shows the competition of which the item is a season \\
subsidiary & P355 & \texttt{[T]} is a subsidiary of \texttt{[H]} . & subsidiary of a company or organization \\
part of & P361 & \texttt{[H]} is part of \texttt{[T]} . & object of which the subject is a part \\
original language of film or TV show & P364 & \texttt{[H]} is the original language of \texttt{[T]}. & language in which a film or a performance work was originally created \\
position held & P39 & \texttt{[H]} holds a position \texttt{[T]} . & subject currently or formerly holds the object position or public office \\
child & P40 & \texttt{[T]} is a child of \texttt{[H]} . & subject has object as child \\
platform & P400 & \texttt{[T]} is a platform of \texttt{[H]} . & platform for which a work was developed or released, or the specific platform version of a software product \\
mouth of the watercourse & P403 & \texttt{[T]} is a mouth of the watercourse of \texttt{[H]} . & the body of water to which the watercourse drains \\
language of work or name & P407 & \texttt{[H]} is written in \texttt{[T]} . & language associated with this creative work (such as books, shows, songs, broadcasts or websites) or a name \\
military rank & P410 & \texttt{[H]}'s military rank is \texttt{[T]} . & military rank achieved by a person, or military rank associated with a position \\
voice type & P412 & \texttt{[H]}'s voice type is \texttt{[T]} . & person's voice type. expected values: soprano, mezzo-soprano, contralto, countertenor, tenor, baritone, bass (and derivatives) \\
position played on team / speciality & P413 & \texttt{[H]} plays the position \texttt{[T]} . & position or specialism of a player on a team \\
original broadcaster & P449 & \texttt{[T]} is the original broadcaster of \texttt{[H]} . & network or service that originally broadcast a radio or television program \\
mountain range & P4552 & \texttt{[T]} is a moutain range of \texttt{[H]} . & range or subrange to which the geographical item belongs \\
said to be the same as & P460 & \texttt{[H]} is said to be the same as \texttt{[T]} . & this item is said to be the same as that item \\
member of & P463 & \texttt{[H]} is a member of \texttt{[T]} . & organization, club or musical group to which the subject belongs. \\
occupant & P466 & \texttt{[T]} is an occupant of \texttt{[H]} . & person or organization occupying property \\
country of origin & P495 & \texttt{[H]} was created in the country \texttt{[T]} . & country of origin of this item (creative work, food, phrase, product, etc.) \\
has part & P527 & \texttt{[H]} has part of \texttt{[T]} . & part of this subject \\
residence & P551 & \texttt{[H]} lives in \texttt{[T]} . & the place where the person is or has been, resident \\
director & P57 & \texttt{[T]} is a director of \texttt{[H]} . & director(s) of film, TV-series, stageplay, video game or similar \\
screenwriter & P58 & \texttt{[T]} wrote the script for \texttt{[H]} . & person(s) who wrote the script for subject item \\
constellation & P59 & \texttt{[H]} is in the constellation \texttt{[T]} . & the area of the celestial sphere of which the subject is a part \\
head of government & P6 & \texttt{[T]} is the head of goverment of \texttt{[H]} . & head of the executive power of this town, city, municipality, state, country, or other governmental body \\
sport & P641 & \texttt{[H]} plays a sport \texttt{[T]} . & sport that the subject participates or participated in or is associated with \\
characters & P674 & \texttt{[T]} is a character of \texttt{[H]} . & characters which appear in this item (like plays, operas, operettas, books, comics, films, TV series, video games) \\
located on terrain feature & P706 & \texttt{[H]} is located on terrain feature \texttt{[T]} . & located on the specified (geo)physical feature. \\
participant & P710 & \texttt{[T]} is a participant in \texttt{[H]} . & person, group of people or organization (object) that actively takes/took part in an event or process (subject) \\
location of formation & P740 & \texttt{[H]} was established in \texttt{[T]} . & location where a group or organization was formed \\
distributed by & P750 & \texttt{[H]} is distributed by \texttt{[T]} . & distributor of a creative work; distributor for a record label; news agency; film distributor \\
notable work & P800 & \texttt{[T]} is notable work of \texttt{[H]} . & notable scientific, artistic or literary work, or other work of significance among subject's works \\
architect & P84 & \texttt{[T]} is an architect of \texttt{[H]} . & person or architectural firm responsible for designing this building \\
composer & P86 & \texttt{[T]} is a composer of \texttt{[H]} . & person(s) who wrote the music \\
main subject & P921 & \texttt{[T]} is the main subject of \texttt{[H]}. & primary topic of a work \\
place served by transport hub & P931 & \texttt{[T]} is a place served by transport hub \texttt{[H]} . & territorial entity or entities served by this transport hub (airport, train station, etc.) \\
work location & P937 & \texttt{[H]} worked in \texttt{[T]} . & location where persons or organisations were actively participating in employment, business or other work \\
tributary & P974 & \texttt{[T]} is a tributary of \texttt{[H]} . & watercourse that flows into an other one \\
successful candidate & P991 & \texttt{[T]} is a successful candidate of \texttt{[H]} . & person(s) elected after the election \\
country & P17 & \texttt{[T]} is a country of \texttt{[H]} . & sovereign state of this item (not to be used for human beings) \\
instance of & P31 & \texttt{[H]} is a \texttt{[T]} . & that class of which this subject is a particular example and member \\
inception & P571 & \texttt{[T]} is created in \texttt{[H]} . & time when an entity begins to exist \\
subclass of & P279 & \texttt{[H]} is a subclass of \texttt{[T]} . & this item is a subclass (subset) of that item \\
capital & P36 & \texttt{[T]} is a capital of \texttt{[H]} . & seat of government of a country, province, state or other type of administrative territorial entity \\
is a list of & P360 & \texttt{[H]} is a list of \texttt{[T]} . & common element between all listed items \\
place of death & P20 & \texttt{[H]} died in \texttt{[T]} . & most specific known (e.g. city instead of country, or hospital instead of city) death location of a person, animal or fictional character \\
place of birth & P19 & \texttt{[H]} was born in \texttt{[T]} . & most specific known (e.g. city instead of country, or hospital instead of city) birth location of a person, animal or fictional character \\
continent & P30 & \texttt{[T]} is the continent of \texttt{[H]} . & continent of which the subject is a part \\
educated at & P69 & \texttt{[H]} studied at \texttt{[T]} . & educational institution attended by subject \\
author & P50 & \texttt{[H]} is written by \texttt{[T]} . & main creator(s) of a written work (use on works, not humans) \\
conflict & P607 & \texttt{[H]} is participated in the battle \texttt{[T]} . & battles, wars or other military engagements in which the person or item participated \\
official language & P37 & \texttt{[T]} is an official language in \texttt{[H]} . & language designated as official by this item \\
facet of & P1269 & \texttt{[H]} is one facet of \texttt{[T]} . & topic of which this item is an aspect, item that offers a broader perspective on the same topic \\
award received & P166 & \texttt{[H]} received an award \texttt{[T]} . & award or recognition received by a person, organization or creative work \\
date of birth & P569 & \texttt{[T]} was born in \texttt{[H]} . & date on which the subject was born \\
influenced by & P737 & \texttt{[H]} is influenced by \texttt{[T]} . & this person, idea, etc. is informed by that other person, idea, etc. \\
employer & P108 & \texttt{[H]} worked for \texttt{[T]} . & person or organization for which the subject works or worked \\
date of death & P570 & \texttt{[T]} died in \texttt{[H]} & date on which the subject died \\
diplomatic relation & P530 & \texttt{[H]} and \texttt{[T]} have diplomatic relations . & diplomatic relations of the country \\
student & P802 & \texttt{[T]} is a student of \texttt{[H]} . & notable student(s) of the subject individual \\
founded by & P112 & \texttt{[H]} is founded by \texttt{[T]} . & founder or co-founder of this organization, religion or place \\
field of this occupation & P425 & \texttt{[T]} is a field of \texttt{[H]} . & field corresponding to this occupation or profession \\
creator & P170 & \texttt{[H]} is created by \texttt{[T]} . & maker of this creative work or other object \\
product or material produced & P1056 & \texttt{[H]} products \texttt{[T]} . & material or product produced by a government agency, business, industry, facility, or process \\
industry & P452 & \texttt{[H]} is in the \texttt{[T]} industry . & specific industry of company or organization \\
family & P53 & \texttt{[H]} is a family of \texttt{[T]} . & family, including dynasty and nobility houses \\
item operated & P121 & \texttt{[H]} operates \texttt{[T]} . & equipment, installation or service operated by the subject \\
named after & P138 & \texttt{[H]} is named after \texttt{[T]} . & entity or event that inspired the subject's name, or namesake \\
given name & P735 & \texttt{[T]} is first name of \texttt{[H]} . & first name or another given name of this person \\
producer & P162 & \texttt{[H]} is produced by \texttt{[T]} . & person(s) who produced the film, musical work, theatrical production, etc. \\
publication date & P577 & \texttt{[T]} is first published in \texttt{[H]} . & date or point in time when a work was first published or released \\
narrative location & P840 & \texttt{[H]} takes place in \texttt{[T]} . & the narrative of the work is set in this location \\
production company & P272 & \texttt{[H]} is produced by studio \texttt{[T]} . & company that produced this film, audio or performing arts work \\
languages spoken, written or signed & P1412 & \texttt{[H]} uses language \texttt{[T]} . & language(s) that a person or a people speaks, writes or signs, including the native language(s) \\
family name & P734 & \texttt{[H]}'s last name is \texttt{[T]} . & part of full name of person \\
organization directed by the office or position & P2389 & \texttt{[H]} is a head of \texttt{[T]} . & organization which is directed by this office \\
connecting line & P81 & \texttt{[H]} is connected to \texttt{[T]} . & railway line(s) subject is directly connected to \\
member of sports team & P54 & \texttt{[H]} is a member of \texttt{[T]} team . & sports teams or clubs that the subject represents or represented \\
part of the series & P179 & \texttt{[H]} is a part of the series \texttt{[T]} . & series which contains the subject \\
parent astronomical body & P397 & \texttt{[H]} is an orbit of \texttt{[T]} . & major astronomical body the item belongs to \\
lyrics by & P676 & \texttt{[T]} wrote the lyrics of \texttt{[H]} . & author of song lyrics \\
different from & P1889 & \texttt{[H]} is different from \texttt{[T]} . & item that is different from another item, with which it may be confused \\
replaces & P1365 & \texttt{[H]} succeeds \texttt{[T]} . & person, state or item replaced \\
sports discipline competed in & P2416 & \texttt{[H]} competed in a \texttt{[T]} sport . & discipline an athlete competed in within a sport \\
drafted by & P647 & \texttt{[H]} was drafted by \texttt{[T]} . & which team the player was drafted by \\
based on & P144 & \texttt{[H]} is based on \texttt{[T]} . & the work(s) used as the basis for subject item \\
opposite of & P461 & \texttt{[H]} is opposite of \texttt{[T]} . & item that is the opposite of this item \\
lowest point & P1589 & \texttt{[H]} is the lowest point of \texttt{[T]} . & point with lowest elevation in the country, region, city or area \\
has quality & P1552 & \texttt{[H]} has characteristic \texttt{[T]} . & the entity has an inherent or distinguishing non-material characteristic \\
use & P366 & \texttt{[H]} is used in \texttt{[T]} . & main use of the subject (includes current and former usage) \\
from narrative universe & P1080 & \texttt{[H]} is featured in universe \texttt{[T]} . & subject's fictional entity is in the object narrative \\
made from material & P186 & \texttt{[H]} is made from \texttt{[T]} . & material the subject or the object is made of or derived from \\
shares border with & P47 & \texttt{[T]} shares border with \texttt{[H]} . & countries or administrative subdivisions, of equal level, that this item borders, either by land or water \\
twinned administrative body & P190 & \texttt{[H]} and \texttt{[T]} are twin cities . & twin towns, sister cities, twinned municipalities and other localities that have a partnership or cooperative agreement, either legally or informally acknowledged by their governments \\
cast member & P161 & \texttt{[T]} is an actor in \texttt{[H]} . & actor in the subject production \\
located on astronomical body & P376 & \texttt{[H]} is on the planet \texttt{[T]} . & astronomical body on which features or places are situated \\ \hline
\caption{Manually built templates used in experiments.}
\label{tab:man_template}
\end{longtable}
\end{small}
\end{center}
